# Supplementary material for: Detection and Quantification of Flow Consistency in Business Process Models
Source: arXiv:1602.02992 source file (2016-02-09)
Supplement: Supplementary file 1 [file appendix-questionnaire-flow.tex]

\section{Questionnaire for the Evaluation of the Flow Consistency}
\label{app:flow-questionnaire}

The following images report all the pages of the questionnaire we used to validate our flow consistency metrics. Each framed box represent one page of the questionnaire.

\begin{center}
	\foreach \x in {1, ..., 15}{
		\fbox{\includegraphics[page=\x,scale=0.4]{img/questionnaire.pdf}} \\[.5em]
		Page \x\ of the questionnaire.\\[2em]
	}
\end{center}
